# Supplementary material for: Proton Gravitational Structure and Mass Decomposition on the Light Front
Source: arXiv:2506.07554 source file (2025-06-09)
Supplement: Supplementary file 1 [file supplemental.pdf]

# Supplemental Material

## I. COMPARISON OF THE PROTON'S $D$-TERM AT $Q^2 = 0$

Figure 1 compares our calculated total proton $D$-term, $D(0) = -3.77 \pm 0.74$, with lattice QCD and other theoretical predictions. Most results are consistent within our uncertainty, particularly the lattice QCD results from the dipole fit [1], which align closely with our calculation.

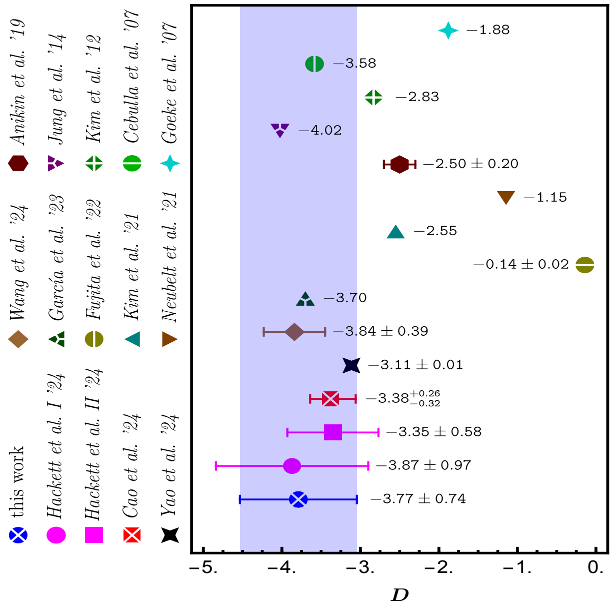


FIG. 1. Comparison of our total proton $D$-term at $Q^2 = 0$ (light blue error band) with lattice QCD calculations from Hackett et al. [1], labeled as "I" (dipole fit) and "II" ($z$-expansion fit), and predictions from other theoretical methods: dispersive analysis (Cao et al. [2]), Faddeev equation (Yao et al. [3]), vector meson photoproduction (Wang et al. [4]), holographic QCD (Fujita et al. [5]), bag model (Neubelt et al. [6]), light-cone sum rules (Anikin et al. [7]), Skyrme models (García et al. [8], Kim et al. [9], Cebulla et al. [10]), and chiral quark soliton models (Kim et al. [11], Goeke et al. [12], Jung et al. [13]).

## II. GRAVITATIONAL FORM FACTORS $B(Q^2)$ AND $J(Q^2)$

Figure 2 presents the gravitational form factors (GFFs) $B(Q^2)$ and $J(Q^2)$ as functions of $Q^2$, separately indicating the quark and gluon contributions. At $Q^2 = 0$, we obtain the values $J_q(0) = 0.27(02)$, $J_g(0) = 0.22(02)$, $J(0) = 0.50(01)$; $B_q(0) = 0.0087(15)$, $B_g(0) = -0.0087(13)$, $B(0) = 0.0000(20)$.

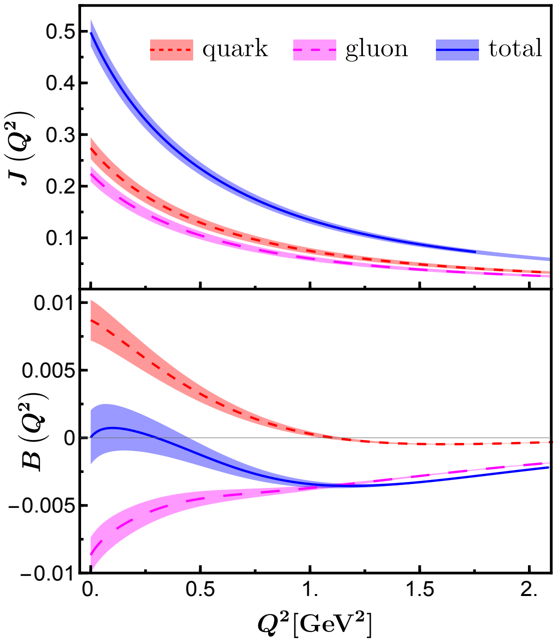


FIG. 2. Proton's GFFs $B(Q^2)$, $J(Q^2) = \left(A(Q^2) + B(Q^2)\right)/2$ and their quark and gluon components as functions of $Q^2$.

## III. PARAMETRIC FITS TO GRAVITATIONAL FORM FACTORS

We fit the GFFs $A(Q^2)$, $D(Q^2)$, and $J(Q^2)$ using a dipole function:

$$f_{\text{dipole}}(Q^2) = \frac{a_0}{(1 + a_1 Q^2)^2}. \tag{1}$$

The resulting fit parameters and reduced chi-square values ($\chi^2_{\text{red}}$) are presented in Table I. The fit quality is evaluated using the reduced chi-square, computed as:

$$\chi^2_{\text{red}} = \frac{1}{N - N_p} \sum_i \frac{(O_i - C_i)^2}{\sigma^2_{\text{tot},i}}, \tag{2}$$

where $N$ is the number of data points, $N_p = 2$ is the number of fit parameters, $O_i$ are the GFF values calculated within our BLFQ framework, $C_i$ are the fitted values, and $\sigma^2_{\text{tot},i}$ represents the total variance obtained by adding the original data uncertainties and propagated fitting uncertainties in quadrature. For reference and comparison, Table II shows the parameters obtained by fitting the same GFFs using a tripole form:

$$f_{\text{tripole}}(Q^2) = \frac{a_0}{(1 + a_1 Q^2)^3}. \tag{3}$$

TABLE I. Dipole fit parameters $a_0$, $a_1$, and reduced $\chi^2_{\rm red}$ for the quark, gluon, and total contributions to the GFFs $A(Q^2)$, $D(Q^2)$, and $J(Q^2)$.

| GFF | $a_0$ | $a_1$ | $\chi^2_{\rm red}$ |
|---|---|---|---|
| $A_q(Q^2)$ | 0.537(40) | 0.900(1) | 0.019 |
| $A_g(Q^2)$ | 0.456(29) | 0.924(11) | 0.046 |
| $A(Q^2)$ | 0.996(11) | 0.910(4) | 1.441 |
| $D_q(Q^2)$ | −1.73(35) | 2.559(10) | 0.056 |
| $D_g(Q^2)$ | −2.04(42) | 1.931(9) | 0.514 |
| $D(Q^2)$ | −3.77(75) | 2.181(0) | 0.276 |
| $J_q(Q^2)$ | 0.273(21) | 0.911(1) | 0.016 |
| $J_g(Q^2)$ | 0.224(15) | 0.932(10) | 0.047 |
| $J(Q^2)$ | 0.499(6) | 0.920(5) | 1.450 |

TABLE II. Tripole fit parameters $a_0$, $a_1$, and reduced $\chi^2_{\rm red}$ for the quark, gluon, and total contributions to the GFFs $A(Q^2)$, $D(Q^2)$, and $J(Q^2)$.

| GFF | $a_0$ | $a_1$ | $\chi^2_{\rm red}$ |
|---|---|---|---|
| $A_q(Q^2)$ | 0.530(40) | 0.528(0) | 1.448 |
| $A_g(Q^2)$ | 0.450(29) | 0.542(6) | 1.146 |
| $A(Q^2)$ | 0.979(49) | 0.534(2) | 2.624 |
| $D_q(Q^2)$ | −1.71(35) | 1.494(6) | 3.928 |
| $D_g(Q^2)$ | −2.01(41) | 1.127(5) | 0.334 |
| $D(Q^2)$ | −3.72(75) | 1.272(0) | 1.307 |
| $J_q(Q^2)$ | 0.270(21) | 0.534(1) | 1.407 |
| $J_g(Q^2)$ | 0.221(15) | 0.547(6) | 1.027 |
| $J(Q^2)$ | 0.490(25) | 0.540(1) | 2.461 |


[1] D. C. Hackett, D. A. Pefkou, and P. E. Shanahan, Phys. Rev. Lett. **132**, 251904 (2024), arXiv:2310.08484 [hep-lat].
[2] X.-H. Cao, F.-K. Guo, Q.-Z. Li, and D.-L. Yao, (2024), arXiv:2411.13398 [hep-ph].
[3] Z. Q. Yao, Y. Z. Xu, D. Binosi, Z. F. Cui, M. Ding, K. Raya, C. D. Roberts, J. Rodríguez-Quintero, and S. M. Schmidt, (2024), arXiv:2409.15547 [hep-ph].
[4] X.-Y. Wang, F. Zeng, and J. Zhang, Chin. Phys. C **48**, 054102 (2024), arXiv:2308.04644 [hep-ph].
[5] M. Fujita, Y. Hatta, S. Sugimoto, and T. Ueda, PTEP **2022**, 093B06 (2022), arXiv:2206.06578 [hep-th].
[6] M. J. Neubelt, A. Sampino, J. Hudson, K. Tezgin, and P. Schweitzer, Phys. Rev. D **101**, 034013 (2020), arXiv:1911.08906 [hep-ph].
[7] I. V. Anikin, Phys. Rev. D **99**, 094026 (2019), arXiv:1902.00094 [hep-ph].
[8] A. Garcia Martin-Caro, M. Huidobro, and Y. Hatta, Phys. Rev. D **108**, 034014 (2023), arXiv:2304.05994 [nucl-th].
[9] H.-C. Kim, P. Schweitzer, and U. Yakhshiev, Phys. Lett. B **718**, 625 (2012), arXiv:1205.5228 [hep-ph].
[10] C. Cebulla, K. Goeke, J. Ossmann, and P. Schweitzer, Nucl. Phys. A **794**, 87 (2007), arXiv:hep-ph/0703025.
[11] J.-Y. Kim, H.-C. Kim, M. V. Polyakov, and H.-D. Son, Phys. Rev. D **103**, 014015 (2021), arXiv:2008.06652 [hep-ph].
[12] K. Goeke, J. Grabis, J. Ossmann, M. V. Polyakov, P. Schweitzer, A. Silva, and D. Urbano, Phys. Rev. D **75**, 094021 (2007), arXiv:hep-ph/0702030.
[13] J.-H. Jung, U. Yakhshiev, and H.-C. Kim, J. Phys. G **41**, 055107 (2014), arXiv:1310.8064 [hep-ph].
